# Supplementary material for: Warm-Inflation: a software for first-principles integration of warm inflation power spectra
Source: arXiv:2610.11880 source file (2026-11-14)
Supplement: Supplementary file 1 [file APPendixB.tex]

\chapter{Gauge invariance: make it more transparent/remove it}\label{app:gauges}
\SetWatermarkText{TO BE DELETED prob}
We will now derive how the scalar components of scalar, vector, and tensor perturbations change upon redefinition of the coordinates on the perturbative level. Starting with the scalars, we first note that for $ f(x)=\bar{f}(x)+\delta f(x)$:
\begin{equation}\label{rules}
    f(x)=\tilde{f}(\tilde{x}) \;\;\;\;\&\;\;\;\;\bar f(\tilde x)=\tilde{\bar f}(\tilde{x})
\end{equation}
The first equality holds as the physical quantity $f$ is being evaluated at the same physical point, and should therefore assume the same value regardless of the choice of the reference frame. The background $\bar f$, however, is just a mathematical reference frame. When we 'pull it back' to the physical manifold $f$, we assign it the same functional form, regardless of the choice of coordinates, hence the second identity. These two conditions together give rise to the transformation rule for a perturbation of a scalar:\footnote{The same result could be obtained by taking the Lie derivative  in an alternative, more mathematically-minded derivation.}
\begin{equation}
    \begin{split}
        \tilde{f}(\tilde x)&=\tilde{\bar{f}}(x+\xi)+\delta \tilde{f}(\tilde{x})\\
        f(x)&=\bar{f}(x+\xi) +\delta \tilde{f}(\tilde{x})\\
        \bar{f}(x)+\delta f(x)&=\bar{f}(x)+\xi^\alpha\partial_\alpha \bar{f}(x) +\delta \tilde{f}(\tilde{x})\\
       \delta \tilde{f}(\tilde x)&= \delta f(x)-\xi^\alpha\partial_\alpha \bar{f}(x)
    \end{split}
\end{equation}
In the first line, we just expanded $\tilde{f}(\tilde x)$, in the second line we've applied \eqref{rules}, in the third line we did two more expansions, while we collected the first-order terms in the last line. We have also dropped order 2 terms in the computation (including a combination of $\xi$ and $\delta$). We can now apply this to our $\delta\varphi$ and $\delta T$ transformations:
\begin{equation}\label{scalars}
    \begin{split}
        \delta\tilde{\varphi}&=\delta\varphi-\xi^0\,\bar{\varphi}'\\
        \delta\tilde{T}&=\delta T-\xi^0\,\bar{T}'
    \end{split}
\end{equation}
Here we've used the fact that the background $\bar{\varphi}$ and $\bar{T}$ only depend on time, and not on space. Right hand-sides are of course evaluated at $\tilde x$ while LHS at $x$, though we suppress these dependancies for brevity. We now move on to the transformation of 4-vectors, starting with their transformation law
\begin{equation}
    \begin{split}
        \tilde{V}(\tilde x)^\alpha&=\frac{\partial \tilde{x}^\alpha}{\partial x^\beta}V(x)^\beta\\
        \tilde{\bar V}( x+\xi)^\alpha+\delta \tilde V(\tilde x)^\alpha&=\left(\delta^\alpha_\beta+\partial_\beta\xi^\alpha\right)\left(\bar V(x)^\beta+\delta V( x)^\beta\right)\\
        \tilde{\bar V}( x)^\alpha+\partial_\mu(\tilde{\bar V}( x)^\alpha)\xi^\mu+\delta \tilde V(\tilde x)^\alpha&=\bar V( x)^\alpha+\delta  V(x)^\alpha+\partial_\beta\xi^\alpha \bar V(x)^\beta\\
        \delta \tilde{V}(\tilde x)^\alpha&=\partial_\beta\xi^\alpha\,\bar V(x)^\beta-\xi^\mu\partial_\mu {\bar V}( x)^\alpha+\delta  V( x)^\alpha
    \end{split}
\end{equation}
In the second line, we've expanded the four vectors, in the third line we expressed $\tilde x$ in terms of $x$ on the LHS, so that in the last line we could use the property that the background quantity's functional form does not change. We again omitted $\mathcal{O}(2)$ terms. We can now apply the result in the last line to our particular 4-vector of interest \eqref{4velocity}, giving us transformation rules for perturbations $v$ and $h_0$:
\begin{equation}\label{vectors}
    \begin{split}
        \delta \tilde{u}^0&=\partial_\beta\xi^0\,\bar u^\beta-\xi^\mu\partial_\mu {\bar u}^0+\delta  u^0\\
        -a^{-1}\tilde{h}_0&=\partial_\tau\xi^0\,(a^{-1})-\xi^0\partial_0 (a^{-1})-a^{-1}h_0\\
        \tilde{h}_0&=-(\xi^0)' \,-\mathcal{H}\,\xi^0+h_0\\
        \\
        \delta \tilde{u}^1&=\partial_\beta\xi^1\,\bar u^\beta-\xi^\mu\partial_\mu {\bar u}^1+\delta  u^1\\
        -a^{-1}\partial_x \tilde v&=\partial_\tau(-\nabla \xi)_x\,a^{-1}-a^{-1}\partial_x v\\
        \tilde v&=\xi'\,+ v\\
    \end{split}
\end{equation}
In the second-to-last line, the subscript $x$ of the divergence of $\xi$ refers to its $x$-component. Lastly, we find a transformation rule for a rank-2 tensor, using the same series of steps as for the 4-vector:
\begin{equation}
    \begin{split}
        \tilde{g}_{\mu\nu}(\tilde x)&=\frac{\partial x^\alpha}{\partial \tilde{x}^\mu}\frac{\partial x^\beta}{\partial \tilde{x}^\nu} \left(\bar g_{\alpha\beta}(x)+\delta g_{\alpha\beta}(x)\right)\\
         \tilde{\bar g}_{\mu\nu}(\tilde x)+ \delta \tilde{g}_{\mu\nu}(\tilde x)&=(\delta^\alpha_\mu-\partial_\mu\xi^\alpha)(\delta^\beta_\nu-\partial_\nu\xi^\beta) \left(\bar g_{\alpha\beta}(x)+\delta g_{\alpha\beta}(x)\right)\\
        \tilde{\bar g}_{\mu\nu}(x)+\partial_\gamma(\tilde{\bar g}_{\mu\nu}(x))\xi^\gamma+ \delta \tilde{g}_{\mu\nu}(\tilde x)&=\bar g_{\mu\nu}(x)+\delta g_{\mu\nu}(x)-\partial_\mu\xi^\alpha \bar g_{\alpha\nu}(x)-\partial_\nu\xi^\beta \bar g_{\mu\beta}(x)\\
        \delta \tilde{g}_{\mu\nu}(\tilde x)&=-\partial_\nu\xi^\beta\,\bar g_{\mu\beta}(x)-\partial_\mu\xi^\alpha\,\bar g_{\alpha\nu}(x)-\xi^\sigma \partial_\sigma \bar g_{\mu\nu}(x)+ \delta g_{\mu\nu}( x)
    \end{split}
\end{equation}
We can now derive the transformation rules for the remaining $h,\,h_D,$ and $\,\vartheta$:
\begin{equation}\label{tensors}
    \begin{split}
        \delta \tilde{g}_{01}&=-\partial_x\xi^0\,\bar g_{00}-\partial_\tau\xi^1\,\bar g_{11}+ \delta g_{01}\\
         \partial_x\tilde{h}&=\partial_x\xi^0-\partial_\tau(-\partial_x \xi)+ \partial_x h\\
         \tilde{h}&=\xi^0+\xi'+  h
        \\\\
        \delta \tilde{g}_{12}&=-\partial_y\xi^1\,\bar g_{11}-\partial_x\xi^2\,\bar g_{22}+ \delta g_{12}\\
        2a^2\partial_x\partial_y\tilde{\vartheta}&=\partial_x\partial_y\xi \,a^2+\partial_x\partial_y\xi\,\,a^2+ 2a^2\partial_x\partial_y\vartheta\\
        \tilde{\vartheta}&=\xi + \vartheta
        \\\\
        \delta \tilde{g}_{11}&=-\partial_1\xi^1\,\bar g_{11}-\partial_1\xi^1\,\bar g_{11}-\xi^0 \partial_\tau \bar g_{11}+ \delta g_{11}\\
        2a^2\left[-\tilde h_D+\left(\partial_x^2-\frac{\nabla^2}{3}\right)\tilde \vartheta(x)\right]&=2\partial_x^2\xi\,a^2-\xi^0 \partial_\tau(a^2)+ 2a^2\left[- h_D(x)+\left(\partial_x^2-\frac{\nabla^2}{3}\right) \vartheta\right]\\
        \tilde h_D &=\xi^0 \mathcal{H}+ h_D-\frac{\nabla^2 \xi}{3}
    \end{split}
\end{equation}
