# Supplementary material for: Warm-Inflation: a software for first-principles integration of warm inflation power spectra
Source: arXiv:2610.11880 source file (2026-11-14)
Supplement: Supplementary file 2 [file code.tex]

\subsection{warm inflation codes}
\begin{enumerate}
    \item SWIM by U. Kumar and S. Das (2026)\\
    \begin{itemize}
        \item \textbf{language}: C++, Python
        \item \textbf{inputs}: $V,\;\Upsilon$
        \item \textbf{output}: power spectrum (for full k?) + constrain model parameters with CMB data 
        \item \textbf{background equations}: no T-dep potential, p and e of radiation fixed
        \item \textbf{perturbation equations}: newtonian gauge... \\
        Their Langevin like ours, but $\varrho=\sqrt{\frac{2\Upsilon T}{a^3}}\;\xi_T+\sqrt{\frac{H^2\sqrt{9+12\pi Q}}{\pi a^3}(1+2n)}\;\xi_Q$. \\
        Their plasma $i$ comp.: the second eq without noise is the same as ours\\
        Their plasma $0$ comp.: not fully compared, but it looks nontrivial\\
        Their EFE: only provide ONE, which matches our $G^0_i$ equation under the assumption their ``momentum perturbation $\psi_R=a(\bar e+\bar p)(h-v)$'' --- why they only provide 1 EFE? There should be 4... Now they only provide 1+1+2 equations in total. Why? 1 is trivial (h0=h0), but the other two? independent from the rest? you get a first order eq for the inflaton term, without the noise - provided their stress tensor is the same as ours.
        \item \textbf{boasts}: full numerical PS for parameter estimation, fast (ML)
        \item \textbf{noise}: ``thermal'' and ``quantum'' noise; thermalization YES/NO; claim $\xi_T$ must be added to stress tensor conservation eq. for stress tensor to be conserved but allow user to leave it out? + thermal part has $2T\Upsilon$, quantum part has bose-einstein distribution, n. \\
        the factor 1/2 may be wrong in their def. of $\chi$, or the factor in front of $\beta$ is wrong in the matrix.
    \end{itemize}
\vspace{1cm}
test it!
\\
    \item WI2Easy (2025)
    \item WarmSPy
    \item Stepping away from the perturbative picture, a plenthora of lattice simulations exist in the literature (\cite{CaravanoCode} mentions a few). However, they have their own shortcomings. For example, \cite{CaravanoCode} while producing fully non-perturbative curvature power spectrum in the cold inflation framework, neglects metric perturbations, motivating it by invoking slow roll, though admitting metric perturbations could still play a role. The code only works during inflation, and does not focus on the subsequent period of reheating. 
\end{enumerate}
