# Supplementary material for: Warm-Inflation: a software for first-principles integration of warm inflation power spectra
Source: arXiv:2610.11880 source file (2026-11-14)
Supplement: Supplementary file 3 [file cosine.tex]

%Here we present the results of the numerical implementation presented in the previous part of the thesis. These include some sample solutions in the weak and strong regime, as well as a parameter scan, followed by an attempt to investigate potential model-independence of our solutions.
%Let us note that while these results were obtained using a specific set of theory parameters, our code can also be used for other models. Some of them are presented Chapter \ref{ch:SM}. 
%\hl{*include a potentially helpful graphic*}



%\chapter{Results}\label{ch:results}
%test case
%\section{Background}
%\section{first-order}
%\subsection{Sample solutions}
%\subsection{Parameter scan and model independence}\label{ch:modelindependence}
%A lot of models of inflation exist (in 2014, over 70 were listed in Encyclopaedia Inflationaris \cite{encyclopedia}). There is a need for a somewhat model-independent treatment. While we cannot provide a truly model independent approach, we try to limit model-dependance in the following ways:



\chapter{Example application: Standard Model with Warm Inflation}\label{ch:SM}
%Inflation and reheating models normally postulate the existence of an (or sometimes multiple) inflaton field(s), just as it is done in this work with $\varphi$. Introducing a new field becomes more attractive if it manages to solve multiple problems in physics at the same time; for example, inflation and the strong CP problem. In this section we quickly recap the strong CP problem and explain how our framework could be applied to a model where the inflaton $\varphi$ is also the QCD axion. The model was proposed by \cite{ZellSM}.

\section{Theoretical foundation}


\subsection{strong CP problem}
Although far from being an expert on QCD, I will still try to summarize some main points relevant to our inflation/reheating research. For details, see for example \cite{ClaudioEncyclopedia} and references therein.\\\\ 
The QCD Lagrangian density includes the matter fields (quarks and gluons), as well as a \textit{theta term}:
\begin{equation}\label{coupling}
   \mathcal{L}\subset  \theta \frac{g^2}{64\pi^2} \epsilon^{\mu\nu\alpha\beta} F^{a}_{\mu\nu} F^a_{\alpha\beta}=  \theta \frac{g^2}{64 \pi^2} F \Tilde{F} 
\end{equation}
QCD field strength tensor is denoted by $F$ and its dual is $\Tilde{F}$. While this term is irrelevant on the classical level (total divergence), on the quantum level it leads to observational consequences. In particular, the term is CP odd and hence leads to CP violation in the strong sector. Experimentally we have, however, found no evidence of CP violation in the strong sector. On the Lagrangian level, this means the $\theta$ term has to be very small. Its magnitude is severely constrained by the electric dipole moment measurements of the neutron. The most stringent bounds on $\theta$ are: \cite{PSIpaperDipoleMoment} $\theta \leq (0\pm 1)\times 10^{-10}$. One could wonder why is $\theta$ so unnaturally small. This is called the strong CP problem.  
\\\\
One cannot, however, set $\theta=0$ a priori by saying CP is a symmetry of the strong sector. This is because of a chiral symmetry. In principle, chiral rotation should be a symmetry, but it leads to a complex rotations of quark masses and a shift in $\theta$ angle. Quark mass matrix comes from the electroweak sector, where CP is not a symmetry, so one cannot impose $\theta\rightarrow0$.
\\\\
A resolution to the strong CP problem is given by Peccei-Quinn symmetry breaking mechanism, where a small value of $\theta$ is generated dynamically. The Peccei-Quinn solution assumes the existence of a $U(1)$ global symmetry in the UV, which is spontaneously broken at some high $\Lambda_{PC}$ scale. As a result, one gets a pseudo Nambu-Goldstone boson called axion $a(x)$. At the same time, the $U(1)$ symmetry is anomalously broken, effectively introducing an extra term in the Lagrangian density: $a(x) \; F\tilde{F}$ through $\theta\rightarrow\theta_{\text{eff}}=\theta+\frac{a(x)}{f_a}$, with $f_a$ making the extra term very much suppressed, compared to the SM scales. Aside from the coupling term, there should be an additional derivative term of $a(x)$ present in the Lagrangian. The derivative term is invariant under a shift symmetry of the axion $a(x)\rightarrow a(x)+\alpha$, however in the broken phase one also has the coupling term, which is not invariant under that global shift symmetry. Axion field $a(x)$ then chooses the value which minimizes the vacuum energy density, which turns out to mean $\theta_{\text{eff}}\rightarrow0$, dynamically solving the strong CP problem.
\\\\
At energies much above $\Lambda_{\text{QCD}}$ scale as well as at the energies much below, expressions for the axion potential can be derived. In the large T regime in dilute gas approximation (from lattice simulations, above $\approx 300$ MeV), the free energy takes form of a cosine, with $\chi(T)$ being the susceptibility:
\begin{equation}
    F(T,\theta)=\chi(T)\left[1-\cos{\theta}\right]
\end{equation}
At zero temperature, the expression becomes proportional to
\begin{equation}
    F(T=0,\theta)\propto \sqrt{1-\frac{4 m_u}{m_d+m_u}\sin{\left(\frac{\theta}{2}\right)}^2}
\end{equation}


\subsection{Potential and dissipation}
\subsection{Potentials for inflation}
slow roll, quantum corrections, steeper potentials allowed by warm inflation
\subsection{older}
\\\\
\textbf{cosine potential, the rise of friction, standard problems of inflation potentials}
\\\\
Above some UV scale, there exists a Lagrangian that includes some kinetic term, and a coupling term like $\varphi G\tilde{G}$. Then, through the symmetry breaking mechanism, the algebra of $G$ is reduced and the Lagrangian changes. A part of the gauge group $G$ generates a cosine-like term, while the other part keeps the coupling $\varphi F\tilde{F}$ where the group structure of $F$ is a subalgebra of that of $G$. Now, varying the Lagrangian with respect to $\varphi$ gives an equation of motion including the stochastic average of $F\tilde{F}$ (the average comes about in case the plasma, described by the gauge group $F$, changes much more rapidly than the inflaton - in that case dt would be considered large, which cannot happen, so we only take into account the avrage behaviour of the plasma, hence the expectation value). The $F\tilde{F}$ term in the equations of motion defines a particular correlator, which can be expanded in the interaction picture. Its expansion can in principle have real and imaginary contributions. In Fourier space, the imaginary component would be associated with a time derivative in real space. Hence, the imaginary part can be written in real space as a coefficient in front of $\dot \varphi$, which can be interpreted as friction ($\Upsilon$). It is then the question for the particular microscopic physics what the explicit expression for $\Upsilon$ is. Aside from the imaginary contribution, the commutator can also have a nonzero real part. This would be interpreted as a correction to the mass (or potential), and could in theory spoil inflation (which can only work with a somewhat restricted set of potentials). In practice, one could impose additional symmetries to the Lagrangian that would forbid diagrams giving rise to large corrections to the mass. \textit{But then Sebsastian \cite{ZellSM} also mentions in his paper that the same diagram gives large corrections to the mass and $\Upsilon$?} For a more detailed explanation on the topic, see \cite{Simona1}.
\\\\
