# Supplementary material for: Warm-Inflation: a software for first-principles integration of warm inflation power spectra
Source: arXiv:2610.11880 source file (2026-11-14)
Supplement: Supplementary file 4 [file initial.tex]

\chapter{Initial conditions}\label{app:InitialConditions}
Choosing initial conditions requires us to quantize a field in a curved background. While the discussion on it can be found in various textbooks and lecture notes (see, for example, \cite{paperreference}, \cite{JPvanderSchaarreference},...), the topic is in itself not trivial. Hence, I will try to didactically present it here as well, and apply it to our specific set up. 
\\\\
As step 0, let us review how to quantize a field in Minkowski space. Then, we shall discuss how our case differs from Minkowski, and what challenges this brings. We further show how our spacetime allows us to circumvent the most pressing challenges and meaningfully define an initial quantum state anyway. Lastly, we present an alternative (but in essence no different) way of determining initial conditions.
\SetWatermarkText{}
\section{Quantizing a field in Minkowski space.}
Consider the action $S=\int d^4x \mathcal{L}$ for a classical field $\chi(\tau,\textbf{x})$:
\begin{equation}
    S=-\frac{1}{2}\int d^4x\left( \partial_\mu \chi(\tau, \textbf{x})\partial^\mu\chi(\tau, \textbf{x})+m^2\chi(\tau, \textbf{x})^2 \right)
\end{equation}
which, upon discarding boundary terms, gives the Klein Gordon equation of motion:
\begin{equation}
    \chi(\tau, \textbf{x})''-\nabla^2\chi(\tau, \textbf{x})+m^2\chi(\tau, \textbf{x})=0
\end{equation}
We now go to Fourier space by doing a plane wave expansion of $ \chi(\tau, \textbf{x})$:\footnote{Since the Klein-Gordon operator is translation invariant, $\textbf{x}$-dependent part of the solution has to obey $f_\textbf{k}(\textbf{x}+\textbf{a})=\lambda_{\mathbf{a}}f_\textbf{k}(\textbf{x})$. This is satisfied by an exponential $f_\textbf{k}(\textbf{x}+\textbf{a})=e^{i\textbf{k}(\textbf{x}+\textbf{a})}=e^{i\textbf{k}\textbf{a}}e^{i\textbf{k}\textbf{x}}=\lambda_{\mathbf{a}}f_\textbf{k}(\textbf{x})$. Exponentials are also eigenfunctions of the momentum operator $\hat{P}_x=-i\partial_x$, so plane wave decomposition is a decomposition in momentum eigenstates.}
\begin{equation}\label{planewave}
    \chi(\tau, \textbf{x})=\int \frac{d^3\textbf{k}}{(2\pi)^{3/2}}\; \chi_\textbf{k}(\tau) e^{i\textbf{k}\cdot\textbf{x}}
\end{equation}
where the mode function obeys
\begin{equation}\label{modefuncteq}
    \chi_\textbf{k}(\tau)''+\omega_k^2\;\chi_\textbf{k}(\tau)=0\;\;,\;\;\;\;\omega_k^2=k^2+m^2
\end{equation}
Let the reader be reminded that $k\equiv|\textbf{k}|$. The above equation is that of a harmonic oscillator with time-independent frequency. Mathematically, the solution is incredibly simple:
\begin{equation}
    \chi_\textbf{k}(\tau)=A_\textbf{k} e^{-i\omega_k\tau}+B_\textbf{k} e^{i\omega_k\tau}
\end{equation}
The solution in physical space thus becomes
\begin{equation}
     \chi(\tau, \textbf{x})=\int  \frac{d^3\textbf{k}}{(2\pi)^{3/2}}\; [A_\textbf{k} e^{-i\omega_k\tau+i\textbf{k}\cdot\textbf{x}}+B_\textbf{-k} e^{i\omega_k\tau-i\textbf{k}\cdot\textbf{x}}] 
\end{equation}
In the second term we changed the variable of integration $\textbf{k}\rightarrow -\textbf{k}$. This is a classical solution. Now we shall quantize it in the standard way: we promote the classical field $\chi(\tau, \textbf{x})$ to a quantum operator $\hat{\chi}(\tau, \textbf{x})$, define its conjugate momentum $\hat{\pi}(\tau,\textbf{x})$, and impose canonical commutation relations. Defining canonical momentum:
\begin{equation}
    \pi(\tau,\textbf{x})\equiv \frac{\partial \mathcal{L}}{\partial\chi(\tau,\textbf{x})'}=\chi(\tau,\textbf{x})'
\end{equation}
Quantizing the field and the canonical momentum:
\begin{equation}
    \hat{\chi}(\tau, \textbf{x})=\int  \frac{d^3\textbf{k}}{(2\pi)^{3/2}}\; [\hat{A}_\textbf{k} e^{-i\omega_k\tau+i\textbf{k}\cdot\textbf{x}}+\hat{B}_\textbf{-k} e^{i\omega_k\tau-i\textbf{k}\cdot\textbf{x}}] \;\;\;\;,\;\;\;\;\;\;\;\;\hat{\pi}=\hat{\chi}(\tau,\textbf{x})'
\end{equation}
Since $\hat{\chi}(\tau, \textbf{x})$ is now an operator, $A_\textbf{k}$ and $B_\textbf{k}$ became operators also. Now, since the operator $\hat{\chi}(\tau, \textbf{x})$ must be self-adjoint, $\hat{A}_\textbf{k}^{\dagger}=\hat{B}_\textbf{-k}$, and consequently $\hat{\chi}(\tau, \textbf{x})=\int  \frac{d^3\textbf{k}}{(2\pi)^{3/2}}\; [\hat{A}_\textbf{k} e^{-i\omega_k\tau+i\textbf{k}\cdot\textbf{x}}+\hat{A}_\textbf{k}^\dagger e^{i\omega_k\tau-i\textbf{k}\cdot\textbf{x}}]$.
\\\\
Imposing canonical commutation relations:
\begin{equation}\label{commiesappendix}
    [\hat{\chi}(\tau, \textbf{x}), \hat{\pi}(\tau,\textbf{y})]\equiv i\delta^{(3)}(\textbf{x}-\textbf{y})\;,\;\;\;[\hat{\chi}(\tau, \textbf{x}), \hat{\chi}(\tau, \textbf{y})]\equiv 0 \;,\;\;\;[\hat{\pi}(\tau,\textbf{x}), \hat{\pi}(\tau,\textbf{y})]\equiv 0
\end{equation}
requires one to establish commutation relations between $\hat{A}_\textbf{k}$ and $\hat{A}_\textbf{k}^\dagger$.\footnote{This is a straightforward procedure: take $\hat{\chi}(\tau, \textbf{x})=\int  \frac{d^3\textbf{k}}{(2\pi)^{3/2}}\; [\hat{A}_\textbf{k} e^{-i\omega_k\tau+i\textbf{k}\cdot\textbf{x}}+\hat{A}_\textbf{k}^\dagger e^{i\omega_k\tau-i\textbf{k}\cdot\textbf{x}}]$ and its time derivative, and commute them in the required 3 ways. Be mindful that each of the terms in commutation relation has their own integration variables; $\textbf{k}$ and $\textbf{h}$ for instance. Recall the integral representation of Dirac delta function.} Here it turns out to be convenient to define $\hat{A}_\textbf{k}=\frac{\hat{a}_\textbf{k}}{\sqrt{2\omega_k}}$ and $\hat{A}_\textbf{k}^\dagger=\frac{\hat{a}_\textbf{k}^\dagger}{\sqrt{2\omega_k}}$, as commutation relations between $\hat{a}_\textbf{k}$ and $\hat{a}_\textbf{k}^\dagger$ then become conventionally normalized:
\begin{equation}\label{commiescreationannihilation}
    [\hat{a}_\textbf{k},\hat{a}_\textbf{h}^\dagger]=\delta^{(3)}(\textbf{k}-\textbf{h})\;\;\;\;\;[\hat{a}_\textbf{k},\hat{a}_\textbf{h}]=[\hat{a}_\textbf{k}^\dagger,\hat{a}_\textbf{h}^\dagger]=0
\end{equation}
with
\begin{equation}\label{chiquantized}
    \hat{\chi}(\tau, \textbf{x})=\int \frac{d^3\textbf{k}}{(2\pi)^{3/2}\sqrt{2\omega_k}}\; [\hat{a}_\textbf{k} e^{-i\omega_k\tau+i\textbf{k}\cdot\textbf{x}}+\hat{a}_\textbf{k}^\dagger e^{i\omega_k\tau-i\textbf{k}\cdot\textbf{x}}] 
\end{equation}
With this in hand, we may define a Hamiltonian $\mathscr{H}$ and rewrite it in terms of operators $\hat{a}_\textbf{k},\hat{a}^\dagger_\textbf{k}$.
\begin{equation}
    \begin{split}
        \mathscr{H}&=\int d^3\mathbf{x}\left[\pi(\tau, \textbf{x})\chi(\tau, \textbf{x})'-\mathcal{L}\right]\\
        &=\frac{1}{2}\int d^3\mathbf{x}\left[\chi(\tau, \textbf{x})'^2+(\nabla \chi(\tau, \textbf{x}))^2+m^2\chi(\tau, \textbf{x})^2\right]\\
        \hat{\mathscr{H}}&=\frac{1}{2}\int d^3\mathbf{x}\int\frac{d^3\mathbf{k}\,d^3\mathbf{h}}{(2\pi)^3 2\sqrt{\omega_k\omega_h}}\left[ \left(-\omega_k\omega_h-k_xh_x-k_yh_y-k_zh_z+m^2\right)\;\left\{\hat{a}_\textbf{k}\hat{a}_\textbf{h} e^{ix_\mu(k^\mu+h^\mu)}+\hat{a}_\textbf{k}^\dagger\hat{a}_\textbf{h}^\dagger e^{-ix_\mu(k^\mu+h^\mu)}\right\} \right.\\
        &\hspace{3cm}\left. +\left(\omega_k\omega_h+k_xh_x+k_yh_y+k_zh_z+m^2\right)\;\left\{\hat{a}_\textbf{k}\hat{a}_\textbf{h}^\dagger e^{ix_\mu(k^\mu-h^\mu)}+\hat{a}_\textbf{k}^\dagger\hat{a}_\textbf{h} e^{-ix_\mu(k^\mu-h^\mu)}\right\} \right]\\
        &=\frac{1}{2}\int\frac{d^3\mathbf{k}}{ 2\omega_k}\left[ \left(-\omega_k^2+k^2+m^2\right)\;\left\{\hat{a}_\textbf{k}\hat{a}_\textbf{k} e^{-2i\omega_k\tau}+\hat{a}_\textbf{k}^\dagger\hat{a}_\textbf{k}^\dagger e^{2i\omega_k\tau}\right\} +\left(\omega_k^2+k^2+m^2\right)\;\left\{\hat{a}_\textbf{k}\hat{a}_\textbf{k}^\dagger +\hat{a}_\textbf{k}^\dagger\hat{a}_\textbf{k} \right\} \right]\\
         &=\frac{1}{2}\int d^3\mathbf{k} \; \omega_k \;\left\{\hat{a}_\textbf{k}\hat{a}_\textbf{k}^\dagger +\hat{a}_\textbf{k}^\dagger\hat{a}_\textbf{k} \right\} \\
         &=\int d^3\mathbf{k} \; \omega_k \;\left[\hat{a}_\textbf{k}^\dagger\hat{a}_\textbf{k}+\frac{1}{2}\delta^{(3)}(\mathbf{0}) \right]
    \end{split}
\end{equation}
The first line is just a definition, in the third we've inserted \eqref{chiquantized} and used a contraction $x_\mu k^\mu=-\omega_k\tau+\mathbf{k}\cdot \mathbf{x}$. Going to the fourth line, we have first recognized delta distributions $\delta^{(3)}(\textbf{...})=\int \frac{d^3\textbf{x}}{(2\pi)^3}e^{i\mathbf{x}\cdot(\textbf{...})}$ and also used them to eliminate the $\int d^3\mathbf{h}$ integrals. In the second-to-last line, we've used the definition of $\omega_k$, followed by the final expression obtained by using commutation relations \eqref{commiescreationannihilation}. Notice the Hamiltonian contains an infinite constant term. This is the vacuum energy. In a non-gravitational QFT, such as in Minkowski case here, we can safely normal order the Hamiltonian, in other words drop the infinite constant (this we cannot do in a gravitational context).
\\\\
At this point we can clarify the meaning of $\hat{a}_\textbf{k},\hat{a}^\dagger_\textbf{k}$. This is most easily done by computing their commutators with the Hamiltonian $ \hat{\mathscr{H}}$, as we know the latter gives the energy of a state. Simple algebra and commutation relations \eqref{commiescreationannihilation} give:
\begin{equation}
    [\hat{ \mathscr{H}},\hat{a}_\mathbf{l}]=\int d^3\mathbf{k}\;\omega_k\left(\hat{a}^\dagger_\textbf{k}\hat{a}_\textbf{k}\hat{a}_\textbf{l}-\left(\left[\hat{a}_\textbf{l},\hat{a}^\dagger_\textbf{k}\right]+\hat{a}^\dagger_\textbf{k}\hat{a}_\textbf{l}\right)\hat{a}_\textbf{k}\right)=-\omega_l \hat{a}_\textbf{l}
\end{equation}
Now, consider the Hamiltonian acting on a state $\ket{\psi}$ that was previously acted on by $\hat{a}_\mathbf{l}$:
\begin{equation}
    \begin{split}
        \hat{ \mathscr{H}}\hat{a}_\mathbf{l}\ket{\psi}&=\left(\hat{a}_\mathbf{l}\hat{ \mathscr{H}}-\omega_l \hat{a}_\textbf{l}\right)\ket{\psi}\\
        &=\left(\hat{a}_\mathbf{l}E-\omega_l \hat{a}_\textbf{l}\right)\ket{\psi}\\
        &=\left(E-\omega_l \right)\hat{a}_\textbf{l}\ket{\psi}
    \end{split}
\end{equation}
We can notice $\hat{a}_\textbf{l}$ lowers the energy of a state by 1 energy quanta. Similarly, one can show the operator $\hat{a}_\textbf{k}^\dagger$ raises the energy of a state. Therefore, we interpret $\hat{a}_\textbf{k}^\dagger$ and $\hat{a}_\textbf{k}$ as creation and annihilation operators respectively. We can use them to define states. Vacuum state $\ket{0}$ is defined as a state with the lowest energy, so lowering its energy should give nothing:
\begin{equation}
    \hat{a}_\textbf{k}\ket{0}=0
\end{equation}
A one-particle with momentum $\textbf{k}$ state is  similarly defined by applying once the creation operator $\hat{a}_\textbf{k}^\dagger$ on the vacuum state: $\hat{a}_\textbf{k}^\dagger\ket{0}=\ket{\textbf{k}}$.  
\\\\\
Let us now return to the quantized, decomposed field $\hat{\chi}(\tau,\textbf{x})$ in \eqref{chiquantized}. A commonly encountered terminology are the notions of \textit{positive frequency} and \textit{negative frequency} modes. Recall that our mode functions need to solve an operator version of \eqref{modefuncteq}, and are thus given by:
\begin{equation}
    \hat{\chi}_\textbf{k}(\tau)= \hat{a}_\textbf{k} u_\textbf{k}(\tau)+\hat{a}_\textbf{k}^\dagger u_\textbf{k}(\tau)^* 
\end{equation}
Where $u_\mathbf{k}(\tau)$ is defined through
\begin{equation}
    u_\textbf{k}(\tau)=\frac{1}{\sqrt{2\omega_k}}e^{-i\omega_k\tau}
\end{equation}
If we apply the time evolution operator $i\partial_\tau$ on both of them, we obtain
\begin{equation}
    i\partial_\tau u_\textbf{k}(\tau)=\omega_k u_\textbf{k}(\tau)\;,\;\;\;\;\;\;i\partial_\tau u_\textbf{k}(\tau)^*=-\omega_k u_\textbf{k}(\tau)
\end{equation}
With $\omega_k>0$, the mode $u_\textbf{k}(\tau)$ is then referred to as a positive frequency mode, while $u_\textbf{k}(\tau)^*$ obtains a minus sign under time evolution, and is thus referred to as negative frequency mode. Positive frequencies thus multiply annihilation operator which defines the vacuum state, while negative frequencies multiply the creation operator.%\footnote{Only requiring mode functions to solve EoM allows a to multiply a combination of creation and annihilation operators. Commutation relations fix normalization, while Hamiltonian shows the constant multiplying positive frequencies should be unambiguosly interpreted as annihilation operator. This can be summarized in a simple prescription: quantize the field $...=...au+a^\dagger u*$, impose commutation relations (=wronskian), and make sure $u$ only contains positive frequencies, if a is to be the annihilation operator. For future: a funny thing happens if u contains both, positive and negative frequency modes.}
\\\\
In Minkowski space there is a unique notion of positive frequency, given by the unique global time translation generator. The positive frequencies then must multiply annihilation operator, which then defines a vacuum state uniquely.% In the contrary, in FRLW spacetime, there is no unique time evolution operator, and hence no unique way to split the solution into positive and negative frequency modes. Hence no unique vacuum.
\newpage
\SetWatermarkText{IN PROGRESS}
\section{Quantizing a field in a curved background. Bunch-Davies vacuum.} 
One can now consider similar analysis in curved spacetime, such as we are dealing with in this thesis. Our background is still homogeneous and isotropic, hence the Fourier mode decomposition \eqref{planewave} still works. However, the FRLW metric explicitly depends on time. What are the consequences of this? Fistly, there is no global timelike Killing vector. Hence, there is no time translation symmetry, and consequently (Noether's theorem) no conserved energy. The Hamiltonian depends on time. Mass term depends on time. Consequently, initially vacuum state can change in a non vacuum state over time (simple example from JPvdS lecture notes). Solution: instantaneous vacuum state. Then 1/sqrt(2 energy) OR: early enough time such that mass loses its time dependence (asymptotically) when we are effectively in Minkowski state. Also solution: 1/sqrt(2k).
\\\\
???
\\\\
... no obvious time evolution operator? In the sense, $i\partial_t$ or $i\partial_\tau$, for instance? Or somehow the annihilation operators evolve in a mix of creation and annihilation operators over time? Is this related to different mode functions satisfying the Wronskian condition (which is just the rewrite of commutation relations?)
\\\\
???
\\\\
Hence, there is no unique way to split the mode functions in positive and negative frequency modes. Recalling \eqref{init}, the only difference to the Minkowski equation of motion for the mode functions \eqref{modefuncteq} is encapsulated in the time dependance of the mass term:
\begin{equation}
    \chi_k(\tau)''+\omega_k(\tau)^2\;\chi_k(\tau)=0\;\;,\;\;\;\;\omega_k(\tau)^2=k^2+m(\tau)^2
\end{equation}

A final comment should be made. In general, the situation in curved spacetime is much more dire than the case we have presented here. We are lucky enough to have a sufficiently symmetric spacetime ....
\\\\
\begin{equation}
     \hat{Q}_{\varphi k}''+k^2\hat{Q}_{\varphi k}=0
\end{equation}
It has 2 solutions, $A e^{-ikt}$ and $B e^{ikt}$. The solution $A e^{-ikt}$ corresponds to the annihilation operator part of the mode expansion, and is referred to as 'positive frequency' solution.\footnote{The split between positive and negative frequencies in general depends on the time coordinate choice and is hence ambiguous. In that case, different observers might see different number of particles in a particular state. However, if different observers are related by isometry transformations, such as Lorentz transformations in Minkowski spacetime, then the split between positive and negative frequencies is unique for that family of observers. That can be achieved if there exists a global time-like killing vector? Otherwise you can still make the split, just it is not unique.}
\\\\
Then, fulfilling canonical commutation relations $[\hat{\chi}_k(\tau),\hat{\chi}_k(\tau)']=i$ or equivalently $\mathcal{W}[u_k,u_k^*]=i$, gives $|c|^2=\frac{1}{2\omega_k}$. Hence,
\begin{equation}
    \hat{\chi}_k(\tau)=u_k(\tau) \,a\, +u_k(\tau)^* a^\dagger\;,\;\;\;\;\;u_k=\frac{1}{\sqrt{2\omega_k}}e^{-i\omega_k\tau}
\end{equation}
When we are in vacuum, we shall only consider the so-called \textit{positive frequency} modes $u_k(\tau)$ associated with annihilation operator. 

\section{Alternative derivation of initial conditions.}
\hl{IN PROGRESS}
\\\\
\begin{equation}
    \chi_k(\tau)''+\omega_k(\tau)^2\;\chi_k(\tau)=0\;\;,\;\;\;\;\omega_k(\tau)^2=k^2+m(\tau)^2
\end{equation}
The mass term is time-dependent, but otherwise this equation would be no different from the field equation in Minkowski space. There are a number of implications of having a time-dependent mass, currently the most relevant being the ambiguity of choosing a vacuum state. For example, unlike in Minkowski vacuum, the energy of $\hat{Q}_{\varphi k}$ is not conserved. Additionally, one may define vacuum to consist of purely \textit{forward-propagating} modes, $e^{-ikx}$, as $w_\textbf{k}\hat{Q}_{ k}(t)e^{i\textbf{k}\cdot\textbf{x}}\ket{0}=0$.
Time changing mass, however, does not have a unique way to define vacuum at all times; positive and negative frequencies mix. We can still define an instantaneous vacuum at early times, when we expect to be in Minkowski vaccuum, and use this as a rule to set initial conditions only. Later it does not matter if forward and backward-propagating solutions mix; that is fine, and can be interpreted as particle production. Just approximating early vacuum as Minkowski allows us to choose a vacuum state and hence set initial conditions. Choosing the forward-propagating modes is the Bunch-Davies prescription.
\\\\




Since \eqref{init} is a second order equation for Fourier mode $\hat{Q}_{\varphi k}$ defined through $\hat{Q}_{\varphi}(x)=\int \frac{dk^3}{(2\pi)^{3/2}}\hat{Q}_{\varphi k}(t)e^{ikx}$, it has 2 solutions. Treating those solutions as plane waves, we can write a mode expansion of a real $\hat{Q}_{\varphi}(x)$ field as a sum of the independent solutions $\hat{Q}_{ k}(t)$ and $\hat{Q}^*_{ k}(t)$:\footnote{We can do that as $k/a \gg H$}
\begin{equation}\label{modeexpansion}
    \hat{Q}_\varphi\equiv \int \frac{d^3\textbf{k}}{\sqrt{(2\pi)^3}}\left[ w_\textbf{k}\hat{Q}_{ k}(t)e^{i\textbf{k}\cdot\textbf{x}}+w_\textbf{k}^\dagger\hat{Q}^*_{ k}(t)e^{-i\textbf{k}\cdot\textbf{x}} \right]
\end{equation}
At this point, $w_\textbf{k}$ and $w_\textbf{k}^\dagger$ are treated just as 2 complex constants of integration. However, in a moment we will perform \textbf{field quantization},  promoting  $w_\textbf{k}$ and $w_\textbf{k}^\dagger$ to annihilation and creation operators respectively.
\\\\
\subsubsection{Wronskian}
A second order differential equation, like \eqref{init}, has 2 integration constant. We will fix one by requiring canonical commutation relations to hold in the early (effectively Minkowski) vacuum. We could immediately start from \eqref{commie3}, but it is also useful to first introduce a Wronskian, an object defined by:
\begin{equation}
    \mathcal{W}[a,b]=ab'-a'b
\end{equation}
Notice the time derivative of a Wronskian between two solutions to \eqref{init} vanishes:
\begin{equation}
\begin{split}
    \mathcal{W}[\hat{Q}_{ k}(t),\hat{Q}_{ k}(t)^*]'&=\hat{Q}_{ k}(t) (\hat{Q}_{ k}(t)^*)''-(\hat{Q}_{ k}(t))''\hat{Q}_{ k}(t)^*\\ &=-(k^2+\hat{m}^2)\left[\hat{Q}_{ k}(t) \hat{Q}_{ k}(t)^*-\hat{Q}_{ k}(t)\hat{Q}_{ k}(t)^*\right]=0
\end{split}
\end{equation}
Evaluating the commutator in vacuum and noting $\mathbf{k}\rightarrow-\mathbf{k}$ (\& $k =|\textbf{k}| $) in third line gives us the value for the Wronskian:
\begin{equation}\label{commie3}
\begin{split}
     [\hat{Q}_\varphi(\textbf{x}),\hat{Q}_\varphi'(\textbf{y})]&=\int \frac{d^3\textbf{k}}{\sqrt{(2\pi)^3}}\int \frac{d^3\textbf{h}}{\sqrt{(2\pi)^3}}\left[ w_\textbf{k}\hat{Q}_{\varphi k}(t)e^{i\textbf{k}\cdot\textbf{x}}+w_\textbf{k}^\dagger\hat{Q}^*_{\varphi k}(t)e^{-i\textbf{k}\cdot\textbf{x}} \right]\left[ w_\textbf{h}\hat{Q}'_{\varphi h}(t)e^{i\textbf{h}\cdot\textbf{y}}+w_\textbf{h}^\dagger\hat{Q}'^*_{\varphi h}(t)e^{-i\textbf{h}\cdot\textbf{y}}\right]\\
     &-\int \frac{d^3\textbf{k}}{\sqrt{(2\pi)^3}}\int \frac{d^3\textbf{h}}{\sqrt{(2\pi)^3}}\left[ w_\textbf{h}\hat{Q}'_{\varphi h}(t)e^{i\textbf{h}\cdot\textbf{y}}+w_\textbf{h}^\dagger\hat{Q}'^*_{\varphi h}(t)e^{-i\textbf{h}\cdot\textbf{y}}\right]\left[ w_\textbf{k}\hat{Q}_{\varphi k}(t)e^{i\textbf{k}\cdot\textbf{x}}+w_\textbf{k}^\dagger\hat{Q}^*_{\varphi k}(t)e^{-i\textbf{k}\cdot\textbf{x}} \right]\\
     &=\int \frac{d^3\textbf{k}}{(2\pi)^3}\left[ \hat{Q}_{\varphi k}\hat{Q}'^*_{\varphi k}\, e^{i\textbf{k}(\textbf{x}-\textbf{y})} -\hat{Q}'_{\varphi k}\hat{Q}^*_{\varphi k}\, e^{-i\textbf{k}(\textbf{x}-\textbf{y})} \right]\\
     &= \int \frac{d^3\textbf{k}}{(2\pi)^3}\mathcal{W}[\hat{Q}_{ k}(t),\hat{Q}_{ k}(t)^*]e^{i\textbf{k}(\textbf{x}-\textbf{y})}\\
     &\overset{!}{=}i\delta^{(3)}(\textbf{x}-\textbf{y})\\
     &\Rightarrow\; \mathcal{W}[\hat{Q}_{ k}(t),\hat{Q}_{ k}(t)^*]=i
\end{split}
\end{equation}
This works at all times. 
\begin{equation}\label{wronskian}
    \mathcal{W}[\hat{Q}_{ k}(t),\hat{Q}_{ k}(t)^*]=\hat{Q}_{\varphi k}\hat{Q}'^*_{\varphi k} -\hat{Q}'_{\varphi k}\hat{Q}^*_{\varphi k}=i
\end{equation}
\\\\
Even after imposing the canonical commutation relations, there is still an ambiguity in how one chooses the mode functions. If $\hat{Q}_{ k}(t)$ and $\hat{Q}_{ k}(t)^*$ solve \eqref{init}, then their linear combination $\hat{\mathcal{\chi}}_k(t)=\alpha \hat{Q}_{ k}(t)+\beta \hat{Q}_{ k}(t)^*$ does so as well.\footnote{$\mathcal{W}[\hat{\mathcal{\chi}}_k(t),\hat{\mathcal{\chi}}_k(t)^*]=(|\alpha|^2-|\beta|^2)\mathcal{W}[\hat{Q}_{ k}(t),\hat{Q}_{ k}(t)^*]$, so if $|\alpha|^2-|\beta|^2=1$ is satisfied, the canonical commutation relations for $\hat{Q}_{ k}(t)$ still hold. One can then alternatively write down a mode expansion $\hat{\mathcal{\chi}}_\varphi\equiv \int \frac{d^3\textbf{k}}{\sqrt{(2\pi)^3}}\left[ a_\textbf{k}\hat{\mathcal{\chi}}_k(t)e^{i\textbf{k}\cdot\textbf{x}}+a_\textbf{k}^\dagger\hat{\mathcal{\chi}}_k(t)^*e^{-i\textbf{k}\cdot\textbf{x}} \right]$ where $a,a^\dagger$ are alternative creation and annihilation operators. One can derive their relations to $w,w^\dagger$ operators. One can use either set of creation and annihilation operators to define different vacua, for example $a\ket{_{(a)}0}=0$ and $w\ket{_{(w)}0}=0$, as well as excited states building orthonormal bases in Hilbert space. However, the vacuum constructed by $a,a^\dagger$ does include particles associated with $w,w^\dagger$, and vice versa. For example, the vacuum expectation value of the number operator of $w$ in $a$ vacuum is $|\beta|^2$ - for details, see \cite{sameasinpaper}. The key tekeaway from this is that the the choice of vacuum and therefore the interpretation of the particle content in the universe depends on the choice of mode functions. The natural question is then whether there exists a preferred set of mode functions that describe the physical vacuum of our theory. From the mathematical point of view, any choice of mode functions is so far equally good. } So, which mode functions ($\hat{\mathcal{\chi}}_k,\hat{\mathcal{Q}}_k,...$) are preferred to describe our physical set up?
\\\\
We choose a particular moment in time, $t_1$. Then, we can define an instantaneous vacuum state, which is the lowest energy state of the Hamiltonian. This can fix our mode functions. Since Hamiltonian depends on time, the state that was the vacuum state at $t_1$ may no longer be the vacuum state at $t_2$, however, this is not a problem, since we set the initial conditions at $t_1$ and later treat the evolution classically. \textit{the hamiltonian trick from Quantum Fields in expanding universe}.
\\\\
Based on \eqref{init}, the Lagrangian at early times is
\begin{equation}
    \mathcal{L}=\int d^3\textbf{x}\left(\frac{1}{2}\hat{\mathcal{Q}}'^{2}_k-\frac{1}{2}(k^2+\hat{m}^2)\hat{\mathcal{Q}}_k^2\right)
\end{equation}
The corresponding Hamiltonian $H(t)=\hat{\mathcal{Q}}'_k(t)\partial_{\hat{\mathcal{Q}}'_k(t)}\mathcal{L}(t)-\mathcal{L}(t)$
\begin{equation}
    H=\int  d^3\textbf{x}\left[ \frac{1}{2}\hat{\mathcal{Q}}'^{2}_k(t)+\frac{1}{2}(k^2+\hat{m}^2)\hat{\mathcal{Q}}_k^2\right]
\end{equation}
Rewriting the Hamiltonian in terms of creation and annihilation operators using \eqref{modeexpansion} ($w,w^\dagger$ are now annihilation and creation operators):
\begin{equation}
    \begin{split}
        H=\int  d^3\textbf{x}\int \frac{d^3\textbf{k}}{(2\pi)^{3/2}}\int \frac{d^3\textbf{h}}{(2\pi)^{3/2}} \left[w_\textbf{k} w_\textbf{h}\left( \hat{\mathcal{Q}}'_k\hat{\mathcal{Q}}'_h +(k^2+\hat{m}^2)\hat{\mathcal{Q}}_k\hat{\mathcal{Q}}_h \right) e^{i\textbf{x}(\textbf{k}+\textbf{h})}\right.\\
        +w_\textbf{k}^\dagger w_\textbf{h}^\dagger\left( \hat{\mathcal{Q}}^{*}_k'\hat{\mathcal{Q}}^{*}'_h +(k^2+\hat{m}^2)\hat{\mathcal{Q}}^{*}_k\hat{\mathcal{Q}}_h^{*} \right) e^{i\textbf{x}(-\textbf{k}-\textbf{h})}\\
        +w_\textbf{k}^\dagger w_\textbf{h}\left( \hat{\mathcal{Q}}^{*}_k'\hat{\mathcal{Q}}'_h +(k^2+\hat{m}^2)\hat{\mathcal{Q}}^{*}_k\hat{\mathcal{Q}}_h \right) e^{i\textbf{x}(-\textbf{k}+\textbf{h})}\\
        \left.+w_\textbf{k} w_\textbf{h}^\dagger\left( \hat{\mathcal{Q}}_k'\hat{\mathcal{Q}}^{*}'_h +(k^2+\hat{m}^2)\hat{\mathcal{Q}}_k\hat{\mathcal{Q}}_h^{*} \right) e^{i\textbf{x}(\textbf{k}-\textbf{h})}\right] \\
        =\int d^3\textbf{k} \left[w_\textbf{k} w_\textbf{-k}\left( \hat{\mathcal{Q}}'_k\hat{\mathcal{Q}}'_k +(k^2+\hat{m}^2)\hat{\mathcal{Q}}_k\hat{\mathcal{Q}}_k \right) +w_\textbf{k}^\dagger w_\textbf{-k}^\dagger\left( \hat{\mathcal{Q}}^{*}_k'\hat{\mathcal{Q}}^{*}'_k +(k^2+\hat{m}^2)\hat{\mathcal{Q}}^{*}_k\hat{\mathcal{Q}}_k^{*} \right) \right.\\
        \left.+w_\textbf{k}^\dagger w_\textbf{k}\left( \hat{\mathcal{Q}}^{*}_k'\hat{\mathcal{Q}}'_k +(k^2+\hat{m}^2)\hat{\mathcal{Q}}^{*}_k\hat{\mathcal{Q}}_k \right) +w_\textbf{k} w_\textbf{k}^\dagger\left( \hat{\mathcal{Q}}_k'\hat{\mathcal{Q}}^{*}'_k +(k^2+\hat{m}^2)\hat{\mathcal{Q}}_k\hat{\mathcal{Q}}_k^{*} \right) \right] \\
        =\int d^3\textbf{k} \left[w_\textbf{k} w_\textbf{-k}\left( \hat{\mathcal{Q}}'_k\hat{\mathcal{Q}}'_k +(k^2+\hat{m}^2)\hat{\mathcal{Q}}_k\hat{\mathcal{Q}}_k \right) +w_\textbf{k}^\dagger w_\textbf{-k}^\dagger\left( \hat{\mathcal{Q}}^{*}_k'\hat{\mathcal{Q}}^{*}'_k +(k^2+\hat{m}^2)\hat{\mathcal{Q}}^{*}_k\hat{\mathcal{Q}}_k^{*} \right) \right.\\
        \left.+(2w_\textbf{k}^\dagger w_\textbf{k}+\delta^{(3)}(\textbf{k}-\textbf{k})\left( |\hat{\mathcal{Q}}_k'|^2 +(k^2+\hat{m}^2)|\hat{\mathcal{Q}}_k|^2 \right)  \right] 
    \end{split}
\end{equation}
In the second line, we recognised delta functions and used them to eliminate $\textbf{h}$ integrals. In the third line, we've used commutation relations for creation and annihilation operators. The vacuum expectation value in $\hat{\mathcal{Q}}_k$ vacuum is then 
\begin{equation}
    \bra{_{\hat{Q}_k}0}H(t_1)\ket{0_{\hat{Q}_k}}=\frac{1}{2}\delta^{(3)}(\textbf{k}-\textbf{k})\int d^3\textbf{k}\left[|\hat{\mathcal{Q}}_k'(t_1)|^2+(k^2+\hat{m}(t_1)^2)|\hat{\mathcal{Q}}_k(t_1)|^2\right]
\end{equation}
The divergent factor reflects the infinite volume. The energy density in the ground state is hence given by 
\begin{equation}
    \varepsilon_{GS}(t_1)=|\hat{\mathcal{Q}}_k'(t_1)|^2+(k^2+\hat{m}(t_1)^2)|\hat{\mathcal{Q}}_k(t_1)|^2
\end{equation}
Since this is a ground state, it's energy should be minimal, which chooses a preferred set of mode functions for our set up. As $\hat{\mathcal{Q}}_k$ is a complex function, we can write it as $\hat{\mathcal{Q}}_k(t)=r_k(t) e^{i\alpha_k(t)}$. The Wronskian condition then gives 
\begin{equation}
    r(t)^2\alpha'(t)=-\frac{1}{2}
\end{equation}
Evaluating the ground state energy now gives
\begin{equation}
    \varepsilon_{GS}(t_1)=r'(t_1)^2+\frac{1}{4r(t_1)^2}+(k^2+\hat{m}(t_1)^2)r(t_1)^2
\end{equation}
Minimizing the instantaneous ground state energy gives initial conditions $r(t_1)'=0$ and $r(t_1)^2=\frac{1}{2\sqrt{(k^2+\hat{m}(t_1)^2)}}$. Consequently, using $\hat{\mathcal{Q}}_k(t)=r_k(t) e^{i\alpha_k(t)}$ parametrization and its derivative we obtain:
\begin{equation}\label{initialQ}
    \hat{\mathcal{Q}}_k(t_1)=\frac{1}{\sqrt{2\sqrt{(k^2+\hat{m}(t_1)^2)}}}\;\;\;\;,\;\;\;\; \hat{\mathcal{Q}}_k'(t_1)=-i\sqrt{k^2+\hat{m}(t_1)^2}\hat{\mathcal{Q}}_k(t_1)
\end{equation}
Here we have set the exponential term to 1, or equivalently $\alpha=0$, as its constant value is arbitrary and unphysical. The obtained functions respect the canonical commutation relations given by the \eqref{wronskian} and at the same time define the instantaneous ground state as a state with minimal energy.\footnote{One can easily check it is a minimum and not maximum by taking second derivatives and noticing they are positive.} This should then be the vacuum state we use to set initial conditions. 
